# Supplementary material for: AG2U -- Autonomous Grading Under Uncertainties
Source: arXiv:2208.02595 source file (2022-08-04)
Supplement: Supplementary file 1 [file 07-appendix.tex]

\section{Appendix}\label{Appendix}
